# Supplementary material for: Trustworthy Deep Learning for Medical Image Segmentation
Source: arXiv:2305.17456 source file (2023-05-27)
Supplement: Supplementary file 1 [file main.tex]

\section{Proofs of \chapref{chap:incompressible}}

\subsection{B-splines notations}
To simplify the notations, let us assume that:
\begin{itemize}
    \item $\Omega=[0,1]^3 \subset \mathds{R}^3$ is the continuous spatial domain of the images,
    \item $k \in \mathds{N}$, the order of the B-splines basis, is less than $3$ (higher order values are rarely used in practice)
    \item $\left(\delta x, \delta y, \delta z\right)= (\frac{1}{n}, \frac{1}{n}, \frac{1}{n})$ is a regular spacing with $n > k$,
    \item $\Omega_{grid}^k$ is a regular grid of knots $\{(x_{i_X}, y_{i_Y}, z_{i_Z})=(\frac{i_X}{n},\frac{i_Y}{n},\frac{i_Z}{n})\}_{i_X,i_Y,i_Z=-k}^{n-1}$ for the spacing $\left(\delta x, \delta y, \delta z\right)$ on $[-\frac{k}{n},1-\frac{1}{n}]^3$.
\end{itemize}
We use the following notations for the B-splines basis functions of order $k$:
\begin{equation*}
    \begin{split}
    \forall i= (i_X, i_Y, i_Z) \in \{-k, \ldots, n-1\}^3, \,\,& \forall \left(x, y, z\right) \in [0,1]^3,\\
        B^k_{i_X,X}(x) =& B^k\left(\frac{x - x_{i_X}}{\delta x} - \frac{k+1}{2}\right)\\
        B^k_{i_Y,Y}(y) =& B^k\left(\frac{y - y_{i_Y}}{\delta y} - \frac{k+1}{2}\right)\\
        B^k_{i_Z,Z}(z) =& B^k\left(\frac{z - z_{i_Z}}{\delta z} - \frac{k+1}{2}\right)\\
    \end{split}
\end{equation*}
where the $B^k$ for $k \in \{0,1,2,3\}$ are defined by:
\begin{equation*}
    \label{eq:bspline}
    \begin{split}
        \forall t \in \mathds{R}, \quad & B^0\left(t\right) = \mathbf{1}_{[-\frac{1}{2}, \frac{1}{2}]}\left(t\right)\\
        & B^1\left(t\right) = \left(1 - |t|\right)\mathbf{1}_{[-1, 1]}\left(t\right)\\
        & B^2\left(t\right) =  \left(\frac{3}{4} - t^2\right)\mathbf{1}_{[-\frac{1}{2}, \frac{1}{2}]}\left(t\right) + \frac{1}{2}\left(\frac{3}{2} - |t|\right)^2\mathbf{1}_{[\frac{1}{2}, \frac{3}{2}]}\left(|t|\right)\\
        & B^3\left(t\right) =\frac{1}{6}\left(4 - 3t^2\left(2 - |t|\right)\right)\mathbf{1}_{[0, 1]}\left(|t|\right) + \frac{1}{6}\left(2 - |t|\right)^3\mathbf{1}_{[1, 2]}\left(|t|\right)\\
    \end{split}
\end{equation*}
Using those notations, in equation \eqref{eq:jac_one_step_error} we define a 3D divergence-conforming SVF $v$ of order $k\geq 2$ and parameters $\left\{(\phi^X_{i}, \phi^Y_{i}, \phi^Z_{i})\right\}_{i \in \{-k, \ldots, n-1\}^3} \in \mathds{R}^{3(n+k)^3}$ as, for all $(x,y,z) \in \Omega$,
\begin{equation*}
    \begin{split}
        % \forall (x,y,z) \in \Omega,\quad 
    v(x,y,z) &= 
    \left(
    \begin{array}{c}
         v^X(x,y,z)  \\
         v^Y(x,y,z) \\
         v^Z(x,y,z)
    \end{array}
    \right)\\
    &= 
    \left(
    \begin{array}{c}
         \sum_{i_X=-k}^{n-1} \sum_{i_Y,i_Z=-(k-1)}^{n-1} B^{k}_{i_X,X}(x) B^{k-1}_{i_Y,Y}(y) B^{k-1}_{i_Z,Z}(z)\,\phi^X_{i_X,i_Y,i_Z}  \\
         \sum_{i_Y=-k}^{n-1} \sum_{i_X,i_Z=-(k-1)}^{n-1} B^{k-1}_{i_X,X}(x) B^{k}_{i_Y,Y}(y) B^{k-1}_{i_Z,Z}(z)\,\phi^Y_{i_X,i_Y,i_Z} \\
         \sum_{i_Z=-k}^{n-1} \sum_{i_X,i_Y=-(k-1)}^{n-1} B^{k-1}_{i_X,X}(x) B^{k-1}_{i_Y,Y}(y) B^{k}_{i_Z,Z}(z)\,\phi^Z_{i_X,i_Y,i_Z}
    \end{array}
    \right)
    \end{split}
\end{equation*}

\subsubsection*{Remark: Support of B-splines basis functions}
The support of a function $f:\mathcal{X} \mapsto \mathds{R}$ is the set of points where $f$ is non-zero, i.e. $\supp\left(f\right) = \left\{x \in \mathcal{X} \,|\, f(x) \neq 0\right\}$.
For any direction $U\in \{X,Y,Z\}$, for $i\in \{-k,\ldots,n-1\}^3$, the support of the function $B^k_{i,U}$ is $]u_i,\, u_i + (k+1)\delta u[$.

%%%%%%%%%%%%%%%%%%%%%%%%%%%%%%%%%%%%%%%%%%%%%%%%%%%%%%%%%%%%%%%
\subsection{Proof of Lemma~\ref{lemma:1}}
In this subsubsection, we give more details on the proof of Lemma~\ref{lemma:1}. 
We start by showing equation \eqref{eq:div_divergence-conforming}.
The functions $B^k$ have the property:
\begin{equation*}
   \forall k \geq 2,\,\, \forall t \in \mathds{R},\quad \dv{B^k}{t} (t) = B^{k-1}\left(t + \frac{1}{2}\right) - B^{k-1}\left(t - \frac{1}{2}\right)
\end{equation*}

\noindent So using the chain rule, we obtain for all $k\geq 2$ and $i = (i_X, i_Y, i_Z) \in \{1, \ldots, N\}^3$,
\begin{equation*}
    \begin{split}
        \dv{B^k_{i,X}}{x} &=\frac{B^{k-1}\left(\frac{x - x_{i_X}}{\delta x} - \frac{k+1}{2} + \frac{1}{2}\right) - B^{k-1}\left(\frac{x - x_{i_X}}{\delta x} - \frac{k+1}{2} - \frac{1}{2}\right)}{\delta x}\\
                    &=\frac{B^{k-1}\left(\frac{x - x_{i_X}}{\delta x} - \frac{k-1+1}{2}\right) - B^{k-1}\left(\frac{x - (x_{i_X}+\delta x)}{\delta x} - \frac{k-1+1}{2}\right)}{\delta x}\\
                    &= \frac{B^{k-1}_{i,X} - B^{k-1}_{(i_X+1,i_Y,i_Z),X}}{\delta x}\\
    \end{split}
\end{equation*}
\noindent Similarly, for the directions $X,Y$ we obtain:
\begin{equation*}
    \begin{split}
        \dv{B^k_{i,Y}}{y} =& \frac{B^{k-1}_{i,Y} - B^{k-1}_{(i_X,i_Y+1,i_Z),Y}}{\delta y}\\
        \dv{B^k_{i,Z}}{z} =& \frac{B^{k-1}_{i,Z} - B^{k-1}_{(i_X, i_Y,i_Z+1),Z}}{\delta z}\\
    \end{split}
\end{equation*}

\noindent Thus, if $k \geq 2$, for all $(x,y,z) \in \Omega=[0,1]^3$:
\begin{equation*}
    \begin{split}
        \pdv{v^X}{x} = \sum_{i_X=-k}^{n-1} \sum_{i_Y,i_Z=-(k-1)}^{n-1} \frac{B^{k-1}_{i_X,X}(x) - B^{k-1}_{i_X+1,X}(x)}{\delta x} B^{k-1}_{i_Y,Y}(y) B^{k-1}_{i_Z,Z}(z)\,\phi^X_{i_X,i_Y,i_Z}\\
    \end{split}
\end{equation*}
Separating the sum into two sums and using the change of index $i_X := i_X + 1$ in the second sum, we obtain:
\begin{equation*}
    \begin{split}
        \pdv{v^X}{x} =& \sum_{i_X=-k}^{n-1} \sum_{i_Y,i_Z=-(k-1)}^{n-1} B^{k-1}_{i_X,X}(x) B^{k-1}_{i_Y,Y}(y) B^{k-1}_{i_Z,Z}(z)\,\frac{\phi^X_{i_X,i_Y,i_Z}}{\delta x}\\
                &- \sum_{i_X=-(k-1)}^{n} \sum_{i_Y,i_Z=-(k-1)}^{n-1} B^{k-1}_{i_X,X}(x) B^{k-1}_{i_Y,Y}(y) B^{k-1}_{i_Z,Z}(z)\,\frac{\phi^X_{i_X-1,i_Y,i_Z}}{\delta x}\\
    \end{split}
\end{equation*}
We have $B^{k-1}_{-k}(x) = B^{k-1}_n(x) = 0$ for all $x \in [0, 1]$
% (see remark in \textbf{1.1})
, so we can group the two sums and we finally obtain:
\begin{equation*}
    \begin{split}
        \pdv{v^X}{x} =& \sum_{i_X,i_Y,i_Z=-(k-1)}^{n-1} B^{k-1}_{i_X,X}(x) B^{k-1}_{i_Y,Y}(y) B^{k-1}_{i_Z,Z}(z)\,\frac{\phi^X_{i_X,i_Y,i_Z}-\phi^X_{i_X-1,i_Y,i_Z}}{\delta x}\\
    \end{split}
\end{equation*}

\noindent Similarly we obtain, for all $(x,y,z) \in \Omega=[0,1]^3$:
\begin{equation*}
    \begin{split}
        \pdv{v^Y}{y} =& \sum_{i_X,i_Y,i_Z=-(k-1)}^{n-1} B^{k-1}_{i_X,X}(x) B^{k-1}_{i_Y,Y}(y) B^{k-1}_{i_Z,Z}(z)\,\frac{\phi^Y_{i_X,i_Y,i_Z}-\phi^Y_{i_X,i_Y-1,i_Z}}{\delta y}\\
        \pdv{v^Z}{z} =& \sum_{i_X,i_Y,i_Z=-(k-1)}^{n-1} B^{k-1}_{i_X,X}(x) B^{k-1}_{i_Y,Y}(y) B^{k-1}_{i_Z,Z}(z)\,\frac{\phi^Z_{i_X,i_Y,i_Z}-\phi^Z_{i_X,i_Y,i_Z-1}}{\delta z}\\
    \end{split}
\end{equation*}

\noindent As a result, for all $(x,y,z) \in \Omega=[0,1]^3$, the divergence of $v$ at $(x,y,z)$ is given by:
\begin{equation*}
    \begin{split}
        \div{v}(x,y,z) =& \sum_{i_X,i_Y,i_Z=-(k-1)}^{n-1} B^{k-1}_{i_X,X}(x) B^{k-1}_{i_Y,Y}(y) B^{k-1}_{i_Z,Z}(z)\,\psi_{i_X,i_Y,i_Z}\\
        \text{s.t.}\quad \forall i_X,i_Y,i_Z,\quad \psi_{i_X,i_Y,i_Z} =& \quad
    \frac{\phi^X_{i_X,i_Y,i_Z} - \phi^X_{i_X-1,i_Y,i_Z}}{\delta x} \\
    &+ \frac{\phi^Y_{i_X,i_Y,i_Z} - \phi^Y_{i_X,i_Y-1,i_Z}}{\delta y}\\
    &+ \frac{\phi^Z_{i_X,i_Y,i_Z} - \phi^Z_{i_X,i_Y,i_Z-1}}{\delta z}
    \end{split}
\end{equation*}

\noindent We are now ready to prove Lemma~\ref{lemma:1}.
Let us assume that $k\geq 2$, and $\mathcal{M}$ is a non-empty subset of $\Omega$. Let $\epsilon \geq 0$
and 
\begin{equation*}
\begin{split}
    \mathbf{J}_{\mathcal{M}}=\{ & (i_X,i_Y,i_Z) \in\{-(k-1),\ldots,n-1\}^3
    \,\,|\,\, \\
    & \left(
    \supp B^{k-1}_{i_X,X} \times \supp B^{k-1}_{i_Y,Y} \times \supp B^{k-1}_{i_Z,Z}
    \right)
    \cap \mathcal{M} \neq \emptyset
    \}
\end{split}
\end{equation*}
\noindent $\mathbf{J}_{\mathcal{M}}$ contains all the indices $(i_X, i_Y, i_Z)$ so that the support of the function $(x,y,z) \mapsto B^{k-1}_{i_X,X}(x) B^{k-1}_{i_Y,Y}(y) B^{k-1}_{i_Z,Z}(z)$ is non-zero for at least one point of $\mathcal{M}$. \medskip

\noindent As a result, if for all $(i_X,i_Y,i_Z) \in \mathbf{J}_{\mathcal{M}},$
\[
    -\epsilon \leq 
    \frac{\phi^X_{i_X,i_Y,i_Z} - \phi^X_{i_X-1,i_Y,i_Z}}{\delta x} +
    \frac{\phi^Y_{i_X,i_Y,i_Z} - \phi^Y_{i_X,i_Y-1,i_Z}}{\delta y} +
    \frac{\phi^Z_{i_X,i_Y,i_Z} - \phi^Z_{i_X,i_Y,i_Z-1}}{\delta z}
    \leq \epsilon,
\]
\noindent Then, for all $(x,y,z) \in \mathcal{M}$,
\begin{equation*}
    \begin{split}
        \abs{\div{v}(x,y,z)} &= \abs{\sum_{i_X,i_Y,i_Z=-(k-1)}^{n-1} B^{k-1}_{i_X,X}(x) B^{k-1}_{i_Y,Y}(y) B^{k-1}_{i_Z,Z}(z)\,\psi_{i_X,i_Y,i_Z}}\\
        &= \abs{\sum_{(i_X,i_Y,i_Z) \in \mathbf{J}_{\mathcal{M}}} B^{k-1}_{i_X,X}(x) B^{k-1}_{i_Y,Y}(y) B^{k-1}_{i_Z,Z}(z)\,\psi_{i_X,i_Y,i_Z}}\\
        &\leq \sum_{(i_X,i_Y,i_Z) \in \mathbf{J}_{\mathcal{M}}} B^{k-1}_{i_X,X}(x) B^{k-1}_{i_Y,Y}(y) B^{k-1}_{i_Z,Z}(z)\,\abs{\psi_{i_X,i_Y,i_Z}}\\
        &\leq \sum_{(i_X,i_Y,i_Z) \in \mathbf{J}_{\mathcal{M}}} B^{k-1}_{i_X,X}(x) B^{k-1}_{i_Y,Y}(y) B^{k-1}_{i_Z,Z}(z)\,\epsilon\\
        &\leq \,\epsilon
    \end{split}
\end{equation*}
Which concludes the proof of Lemma~\ref{lemma:1} $\blacksquare$

%%%%%%%%%%%%%%%%%%%%%%%%%%%%%%%%%%%%%%%%%%%%%%%%%%%%%%%%%%%%%%%
\subsection{Proof for Lie exponential approximation and incompressibility}

\noindent In this subsubsection, we give a detailed proof for the error of incompressibility with an Euler approximation of the Lie exponential (8).
\noindent Let $K \in \mathds{N}$, let $\tau = \frac{1}{2^K}$ be the time step in the Euler integration.
The Euler approximation of the Lie exponential for the time step $\tau$ is given by:
\begin{equation*}
    \begin{split}
        \widetilde{\exp} &= \left(I + \frac{1}{2^K}v\right) \circ \ldots \circ \left(I + \frac{1}{2^K}v\right)\\
            &= \left(I + \frac{1}{2^K}v\right)^{2^K}
    \end{split}
\end{equation*}
where $I$ is the identity mapping.

\noindent Let $\mathcal{M}$ be a non-empty subregion of the spatial domain $\Omega$ and $m=(m_X,m_Y,m_Z) \in \mathcal{M}$.
The Jacobian of the first step of the Euler integration $\left(I + \frac{1}{2^K}v\right)$ at $m$ is given by:
\begin{equation*}
    \begin{split}
        \det\left(J_{I + \frac{1}{2^K} v}(m)\right) &= 
            \left|
            \begin{array}{ccc}
                \frac{1}{2^K}\pdv{v^X}{x}(m) + 1 & \frac{1}{2^K}\pdv{v^X}{y}(m)     & \frac{1}{2^K}\pdv{v^X}{z}(m)\\
                \frac{1}{2^K}\pdv{v^Y}{x}(m)     & \frac{1}{2^K}\pdv{v^Y}{y}(m) + 1 & \frac{1}{2^K}\pdv{v^Y}{z}(m)\\
                \frac{1}{2^K}\pdv{v^Z}{x}(m)     & \frac{1}{2^K}\pdv{v^Z}{y}(m)     & \frac{1}{2^K}\pdv{v^Z}{z}(m) + 1\\
            \end{array}
            \right|\\
            &=1 + \frac{1}{2^K} \div{v}(m) + \mathcal{O}\left(\left(\frac{1}{2^K}\right)^2\right)
    \end{split}
\end{equation*}
Let us note:
\begin{equation*}
\left\{
    \begin{aligned}
        m_0 &= m\\
    \forall k \in \{1, \ldots, 2^K\}, \quad m_k &= \left(I + \frac{1}{2^K}v\right)(m_{k-1})\\
        &= \left(I + \frac{1}{2^K}v\right)^{k}(m)
    \end{aligned}
\right.
\end{equation*}
Using the chain rule and the fact that the determinant of the composition of two matrices is equal to the product of their determinant, we obtain:
\begin{equation*}
    \begin{split}
        \det\left(J_{\widetilde{exp}(v)}(m)\right) &= \det\left(J_{\left(I + \frac{1}{2^K} v\right)^{2^K}}(m)\right)\\
        &= \det\left(J_{\left(I + \frac{1}{2^K} v\right) \circ \left(I + \frac{1}{2^K} v\right)^{2^K - 1}}(m)\right)\\
        &= \det\left(J_{\left(I + \frac{1}{2^K} v\right)}(m_{2^K - 1})\right)\det\left(J_{\left(I + \frac{1}{2^K} v\right)^{2^K - 1}}(m)\right)\\
        &= \prod_{k=0}^{2^K-1} \det\left(J_{I + \frac{1}{2^K} v}(m_k)\right)\\
        &= \prod_{k=0}^{2^K-1} \left(1 + \frac{1}{2^K} \div{v}(m_k) + \mathcal{O}\left(\left(\frac{1}{2^K}\right)^2\right)\right)\\
        &= 1 + \frac{1}{2^K}\left(\sum_{k=0}^{2^K-1} \div{v}(m_k)\right) + \mathcal{O}\left(\frac{1}{2^K}\right)
    \end{split}
\end{equation*}

\noindent Let us now assume that $v$ satisfies the condition of Lemma \ref{lemma:1} for $\epsilon$ close to $0$, up to machine precision (typically $\epsilon=\epsilon_{mach}=10^{-16}$).
If in addition, $\forall k \in \{0, \ldots, 2^K - 1\}, m_k \in \mathcal{M}$.
Then, $\forall k \in \{0, \ldots, 2^K - 1\}, \abs{\div{v}(m_k)} \leq \epsilon_{mach}$, and
\begin{equation}
    \label{eq:ineq_error}
    \abs{\frac{1}{2^K}\left(\sum_{k=0}^{2^K-1} \div{v}(m_k)\right)} \leq \frac{1}{2^K}\left(\sum_{k=0}^{2^K-1} \abs{\div{v}(m_k)}\right) \leq \epsilon_{mach}
\end{equation}

\noindent As a result, we obtain the approximation given in \eqref{eq:jac_error}:
\begin{equation*}
    \det\left(J_{\widetilde{exp}(v)}(m)\right) = 1 + \mathcal{O}\left(\tau + \epsilon_{mach}\right) \quad\blacksquare
\end{equation*}

\subsubsection*{Remark: divergence-free SVF does not guarantee incompressibility of the transformation when $\mathcal{M}$ is local and the deformation is large}
In the case at least one of the $m_k$ is outside of $\mathcal{M}$, inequalities \eqref{eq:ineq_error} do not hold anymore.
Although the divergence of the SVF $v$ is uniformly close to $0$ on $\mathcal{M}$, some point can be deformed in a compressible manner.
This happens when the deformation is large and points that were initially inside $\mathcal{M}$ end up outside of $\mathcal{M}$ during the Euler integration.
In practice, deviations from an incompressible deformation in $\mathcal{M}$ can be observe for accurate divergence-free SVFs in $\mathcal{M}$, as illustrated in Fig.~\ref{fig:ssfp_boxplot}.

Fortunately, the definition of $J_{\mathcal{M}}$ implies the presence of margins around the incompressible region $\mathcal{M}$.
As a consequence, inequalities \eqref{eq:ineq_error} are verified in practice for small and moderate deformations in $\mathcal{M}$, as illustrated in Fig.~\ref{fig:logJacobian}.
One can verify that thoses margins are linear in the order $k$ of the B-splines basis.

It is worth noting that this limitation is due to the use of SVFs, also used in previous works.
In addition, when $\mathcal{M}$ is equal to the entire image domain $\Omega$, inequalities \eqref{eq:ineq_error} are always satisfied for a divergence-free SVF obtained by our method.
